# Supplementary material for: SAMPL9 blind predictions using nonequilibrium alchemical approaches
Source: arXiv:2202.06720 source file (2022-02-14)
Supplement: Supplementary file 1 [file SI.pdf]

# Supporting Information for "SAMPL9 blind predictions using nonequilibrium alchemical approaches"

Piero Procacci*,† and Guido Guarnieri‡

†*Dipartimento di Chimica "Ugo Schiff", Universit degli Studi di Firenze, Via della Lastruccia 3, Sesto Fiorentino, I-50019 Italy*

‡*ENEA, Portici Research Centre, DTE-ICT-HPC, P.le E. Fermi, 1, I-80055 Portici Italy*

E-mail: procacci@unifi.it

Work distribution of the bound state (red), unbound state (blue) and of the convolution (black) for the thirteen host-guest system in SAMPL9 and for the additional ligands for pre-assessment (see main text). The bound and unboud state work values have been obtained running 360 trajectories lasting 1,44 ns and 0.36 ns, respectively.

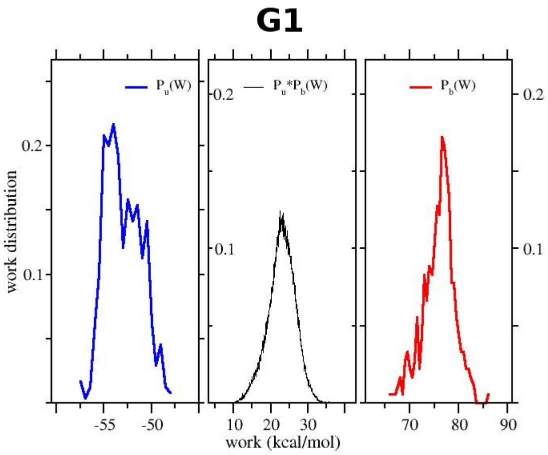

## G2

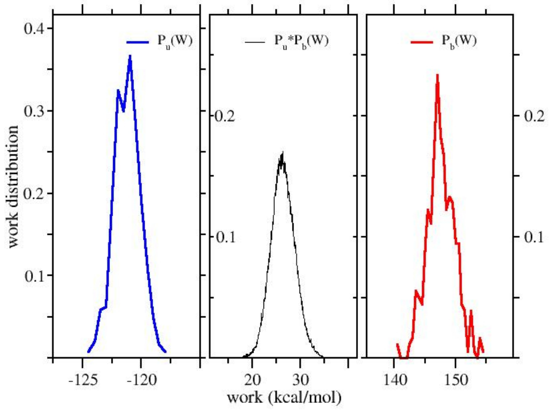

P_u(W)
P_u*P_b(W)
P_b(W)
work distribution
work (kcal/mol)


## G3

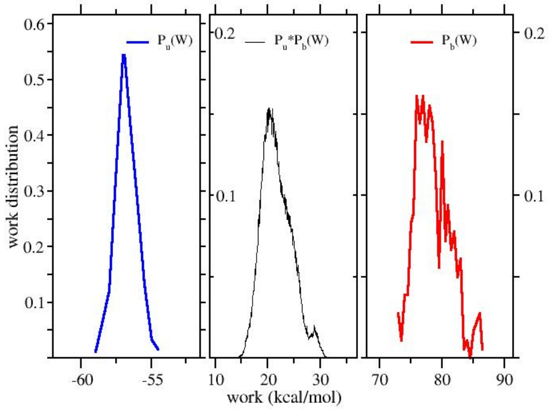

P_u(W)
P_u*P_b(W)
P_b(W)
work distribution
work (kcal/mol)


## G4

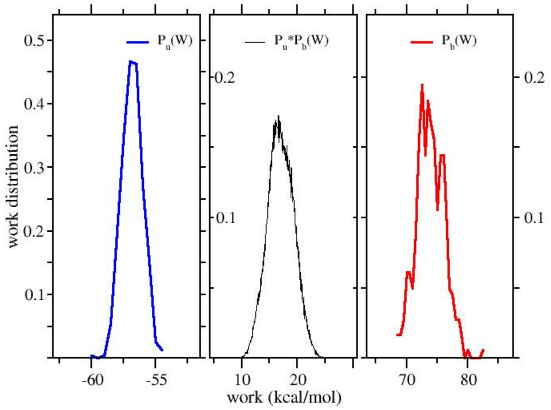

P_u(W)
P_u*P_b(W)
P_b(W)
work distribution
work (kcal/mol)

# G5

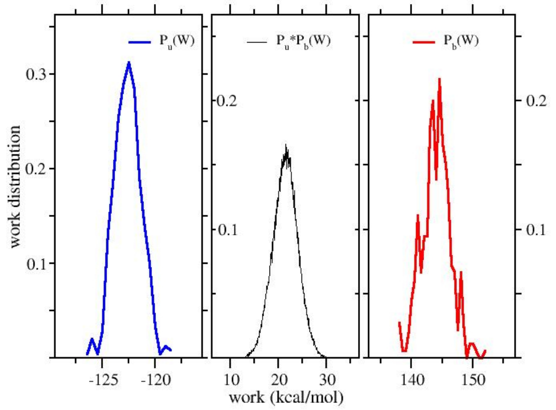

P_u(W)
P_u*P_b(W)
P_b(W)
work distribution
work (kcal/mol)


# G6

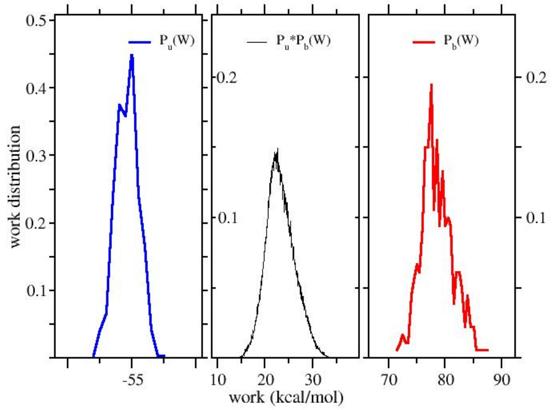

P_u(W)
P_u*P_b(W)
P_b(W)
work distribution
work (kcal/mol)


# G7

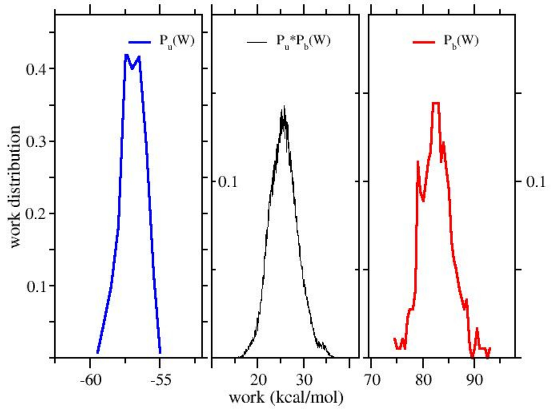

P_u(W)
P_u*P_b(W)
P_b(W)
work distribution
work (kcal/mol)

**G8**

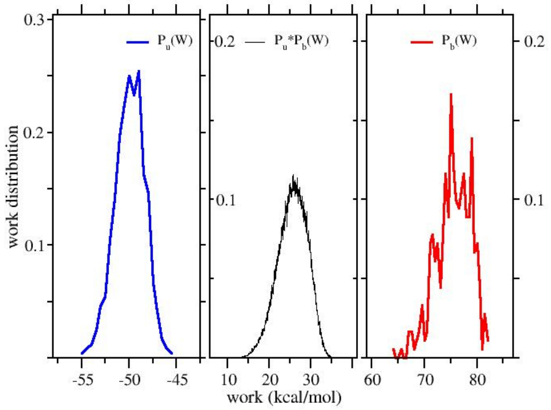

P_u(W)
P_u*P_b(W)
P_b(W)
work distribution
work (kcal/mol)


**G9**

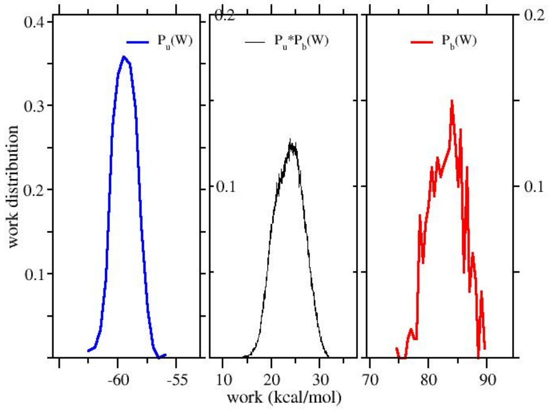

P_u(W)
P_u*P_b(W)
P_b(W)
work distribution
work (kcal/mol)


**G10**

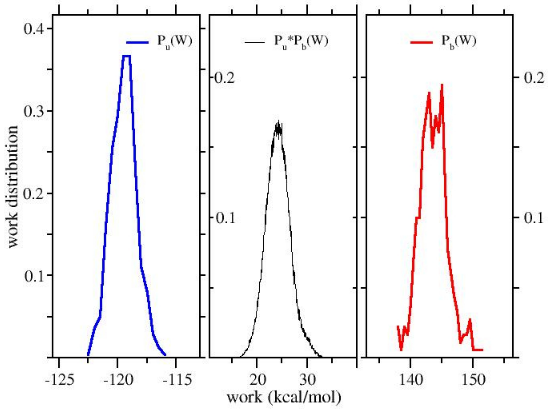

P_u(W)
P_u*P_b(W)
P_b(W)
work distribution
work (kcal/mol)

**G11**

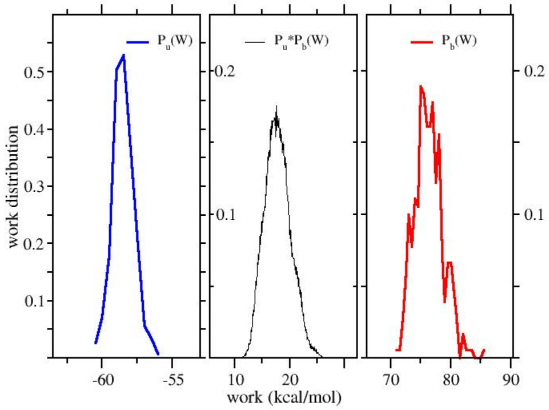

$P_u(W)$
$P_u*P_b(W)$
$P_b(W)$
work distribution
work (kcal/mol)


**G12**

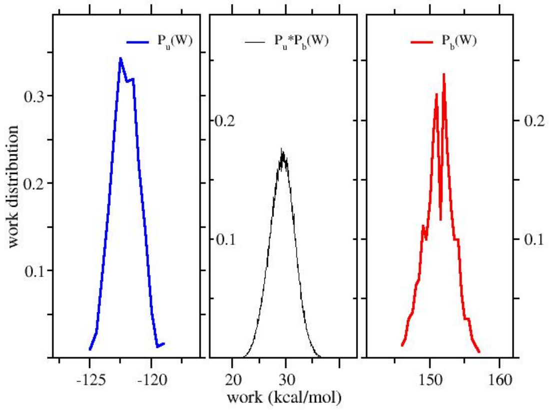

$P_u(W)$
$P_u*P_b(W)$
$P_b(W)$
work distribution
work (kcal/mol)


**G13**

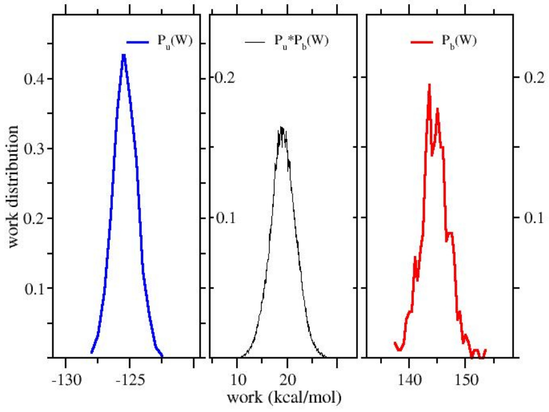

$P_u(W)$
$P_u*P_b(W)$
$P_b(W)$
work distribution
work (kcal/mol)

G14

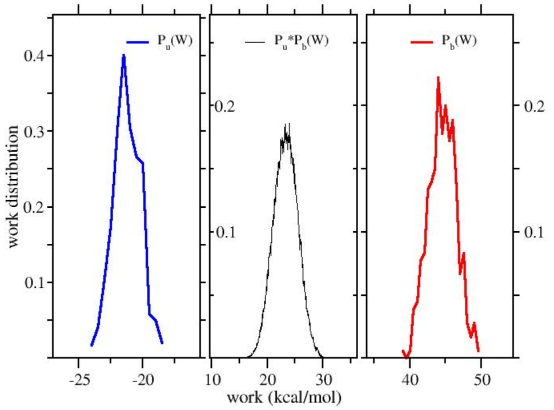
work distribution
Pu(W)
Pu*Pb(W)
Pb(W)
work (kcal/mol)

G15

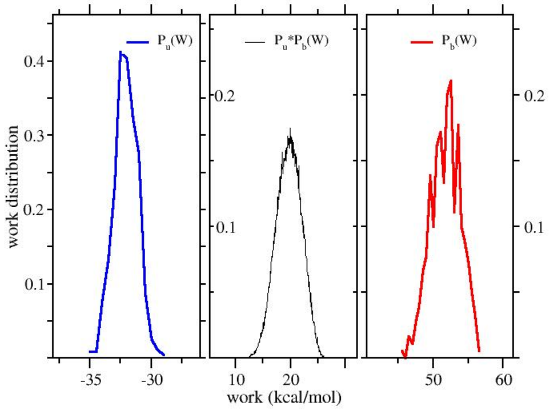
work distribution
Pu(W)
Pu*Pb(W)
Pb(W)
work (kcal/mol)

G16

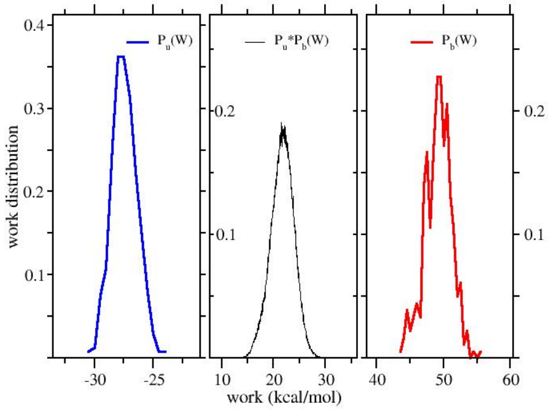
work distribution
Pu(W)
Pu*Pb(W)
Pb(W)
work (kcal/mol)

G17

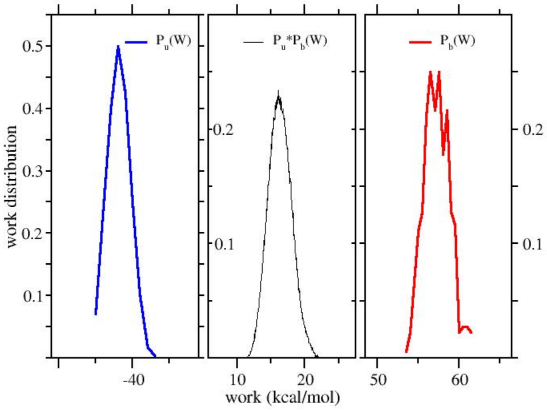
P_u(W)
P_u*P_b(W)
P_b(W)
work distribution
work (kcal/mol)

G18

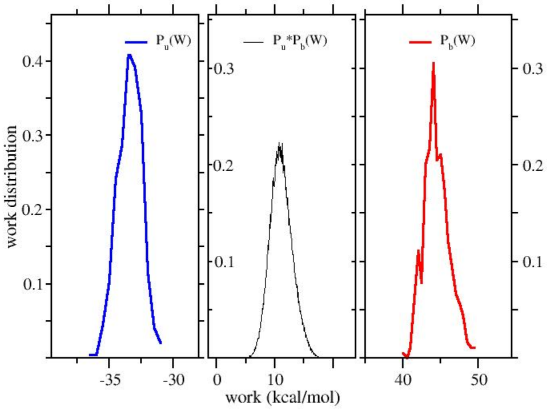
P_u(W)
P_u*P_b(W)
P_b(W)
work distribution
work (kcal/mol)
